# Supplementary material for: Flow-Induced Shift of the Donnan Equilibrium for Ultra-Sensitive Mass Transport Measurement Through a Single Nanochannel
Source: arXiv:1910.13126 source file (2019-10-29)
Supplement: Supplementary file 1 [file SuppMatFlowInducedShift.pdf]

# Supplementary material for "Flow-induced shift of the Donnan equilibrium for ultra-sensitive mass transport measurement through a single nanochannel"

Simon Gravelle[1,2] and Christophe Ybert[1]

[1] *Univ Lyon,Université Claude Bernard Lyon1, CNRS, Institut Lumière Matière, F-69622 Villeurbanne, France*

[2] *School of Engineering and Material Science, Queen Mary University of London, UK*

(Dated: September 26, 2019)

**CONTENTS**

I. Experiment 2
A. Fabrication details 2
B. Method 2
C. Mass flow estimate 3
D. Signal treatment 3
E. Impact of surface adsorption 4

II. One-dimensional analytical calculation with explicit description of the transition zones 4

III. Two-dimensional analytical calculation 7
A. Calculation of $\alpha_{2D}$ 8

IV. Finite element calculations 9
A. System 10
B. Hydrodynamics 10
C. Electrostatics 10
D. Transport of diluted species for salt 11
E. Transport of diluted species for dye 11
F. Validity of the zero-Peclet assumption for salt 11

V. Effect of reversible adsorption on detection resolution 12

References 12

# I. EXPERIMENT

## A. Fabrication details

Slit micro-nanochannels are realized by standard clean-room fabrication, the fabrication protocol follows closely the one detailed in Chauvet et al. [1]. In short, the micro-nanodevices are fabricated using silicon chips with nanochannels bridging between two side microchannels. The lateral dimensions of the channels are designed on a photomask, and both nanochannels (150 nm in depth, 5 µm in width and either 25 µm or 500 µm in length) and microchannels (10 µm in depth and 200 µm in width) are etched in silicon by reactive ion etching (ICP omega 201 machine). The surface is electrically insulated with a 100 nm thick silicon oxide layer grown by thermal oxidation. Sealing of the silicon wafer to a glass substrate (170 µm thick) is ensured by anodic bonding and holes are drilled by sand blasting at microchannels ends.

## B. Method

The microchannels serve as two reservoirs separated by the nanochannel slit, with both reservoirs containing the same solution. For the solution, we used Rhodamine 6G (R6G), a monovalent cationic dye in aqueous solution, prepared in potassium chloride (KCl) solutions with different dilutions ($10^{-4}$ to $10^{-2}$ M) in deionized water (18 MΩ·cm).

The nanofluidic system is inserted in a Fluorescence Correlation Spectroscopy homemade setup. This setup is based on an inverted microscope with water immersion objective (60x, NA = 1.2) with a confocal illumination and detection pathway. Fluorescence is excited with a focused laser beam ($\lambda_{ex.} = 532$ nm), and the signal emitted by the dyes inside the confocal volume of 500 nm diameter localized inside the channel is filtered by a confocal pinhole and split before collection by two avalanche photodiodes. The power of the laser was chosen to be low enough to have no significant impact on the measurement through photobleaching. From the measurement of the typical adsorption duration $\tau_{\mathrm{ads}}$ at varying laser power (Fig. S1 B), we choose $P = 40$ µW.

Unless otherwise stated, the confocal volume was located at the center $x = 0$ of the channel. The pressure drop $\Delta p$ between the two sides of the channel was varied using a pressure controller (ElveFlow) or using gravity, between 0 and 400 mbar, with a minimal increment of $(1 \pm 0.1)$ mbar.

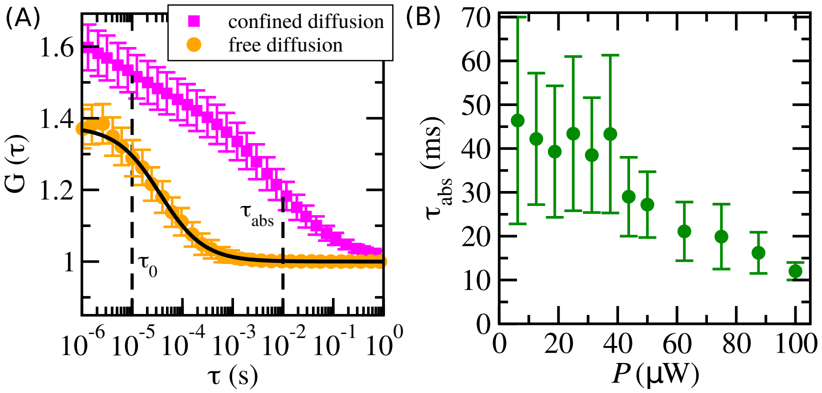


FIG. S1. (A) Fluorescence intensity correlation function $G(\tau)$. (Orange): recorded in bulk, *i.e.* with a confocal volume located far from any surface; (Pink): recorded in confined environment, *i.e.* within a nanochannel in the vicinity of adsorbing surfaces; Vertical dash lines: signal characteristic time scales: the free diffusion time scale $\tau_0$ present in both cases, and the additional time scale $\tau_{\rm ads}$ appearing only near surfaces as a signature of the dye reversible adsorption at the wall. Variation of the time scale $\tau_{\rm ads}$ associated with the reversible adsorption of the dyes at the wall with the power of the laser $P$.

### C. Mass flow estimate

From the value of the applied pressure drop $\Delta p$, the flow rate $Q$ through the channel was estimated using Poiseuille's law as

$$Q = \frac{wh^3}{12\eta L} \times \Delta p, \tag{1}$$

with $\eta = 1\,$mPa.s the water viscosity. Note that in the present configuration, all the pressure drop occurs between the nanochannel ends, with the connecting microchannels hydrodynamic resistance being negligible. Alike, departures from eq. (1) due to hydrodynamics entrance dissipation [2, 3] have been discarded as it reaches at worst $1\,\%$ in the present system, as checked by finite element calculations performed in the same spirit as in reference [4]. The mean velocity of the flow $u$ was then estimated as $u = Q/hw$, and the Peclet number as $\mathrm{Pe} = uL/D$ with $D$ the coefficient diffusion of the dye, here Rhodamine 6G.

### D. Signal treatment

The collected signal $I(t)$ is statistically treated by autocorrelation analysis [5]

$$G(\tau) = \frac{\langle I(t) I(t+\tau)\rangle}{\langle I(t)\rangle^2}. \tag{2}$$

Note than in practice, the signal is initially split onto two Avalanche Photodiode Detectors (APDs) and cross-correlated in order to eliminate the after-pulsing correlation signal from a single detector [6].

The resulting correlation curve yields a measure of self-similarity of the system after a certain lag time, and its amplitude describes the normalized variance of the fluorescence fluctuations, see examples in Fig. S1 A. When performed in a bulk solution, *i.e.* far from any surface, the correlation function reveals one single characteristic time $\tau_0$, and is well fitted by classical expectations for dye diffusion

$$G(\tau) = \frac{1}{n_0}\left(1 - \tau/\tau_0\right)^{-1} + 1, \tag{3}$$

where $\tau_0 = w_{xy}^2/(4D)$ and $w_{xy}$ is the lateral size of the measurement box, $n_0$ the average number of dye molecules in the measurement volume.

On the other hand, when the measurement is performed near solid surfaces, as is the case inside nanochannels, a second characteristic time $\tau_{\rm ads} \sim 10\,$ms appears. It is the signature of the dye reversible adsorption on the channel

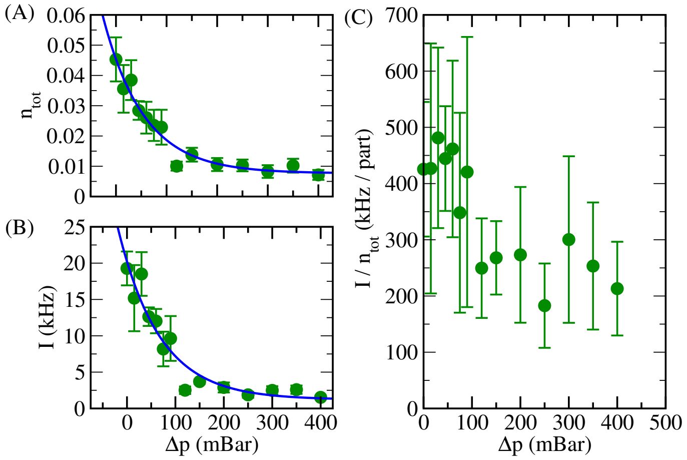


FIG. S2. Nanochannel probe concentration and fluorescence intensity under flow. (A): Total probe number within the confocal volume as extracted from correlation function, as a function of the applied pressure difference (channel of length L=25 µm and $c_s = 10\,\mathrm{mM}$). Solid line: fit according to $y = a\exp(-bx) + c$, with $b = 0.12\,\mathrm{mBar}^{-1}$. (B): Total fluorescence intensity corresponding to data in (A). Solid line: fit according to $y = a\exp(-bx) + c$, with $b = 0.11\,\mathrm{mBar}^{-1}$. (C): Intensity per probe for data in (A).

surface [7–10]. Note that the impact of the reversible adsorption on the correlation function is known and some expression taking into account the existence of both adsorbed and free populations exists [10]. However, in the following we will be only interested in the probe concentration inside the channel rather than in the correlation time scales, and the only information we extract from the correlation functions is the total number of probes in the detection volume defined as

$$n_{\text{tot}} = \frac{1}{G(\tau = 1\,\mu s) - 1}. \tag{4}$$

From the average number of probe, the concentration $c = n_{\text{tot}}/V_d$ is calculated, where $V_d$ is the detection volume $V_d = \pi w_{xy}^2\, h$. Note that the total number of probes $n_{\text{tot}}$ at a given point inside the nanochannel evolves qualitatively proportionally with the average collected intensity $\langle I(t)\rangle$, see Fig. S2 A-B, with however the ratio of intensity per probe that slightly decreases for increasing pressure difference, see Fig. S2 C.

### E. Impact of surface adsorption

As previously stated, autocorrelation functions obtained from measurements performed inside the nanochannel show the existence of two regimes with respective characteristic times $\tau_0$ and $\tau_{\text{ads}}$, see Fig. S1 A and Fig. 1 (main). The two characteristic times are well separated from each other, exist regardless of the convection, and are the signature of the presence of two dye populations: a surface population with slower diffusion due to reversible dye adsorption on the solid surface [7–10], and a bulk population with associated free-dye diffusivity.

For the present mass flow measurement to be accurate, one has to make sure that the existence of a "slow population" aside the "normal population" does not impact the resolution of the method. It is found that, when normalized, curves obtained at various pressure differences collapse into a single one, which indicates that the two populations evolve proportionally to each other, see the insert of Fig. 1 (main). This means that both populations are in equilibrium with each other, and that the measurement can be performed indifferently in presence and in absence of surface adsorption, which makes the present method applicable to most surfaces and dyes.

## II. ONE-DIMENSIONAL ANALYTICAL CALCULATION WITH EXPLICIT DESCRIPTION OF THE TRANSITION ZONES

The present calculation focuses on the concentration profile of a charged probe inside a one dimensional channel of length $L$ with attractive electrostatic potential $V_D$. Each end of the channel is in contact with large reservoirs of

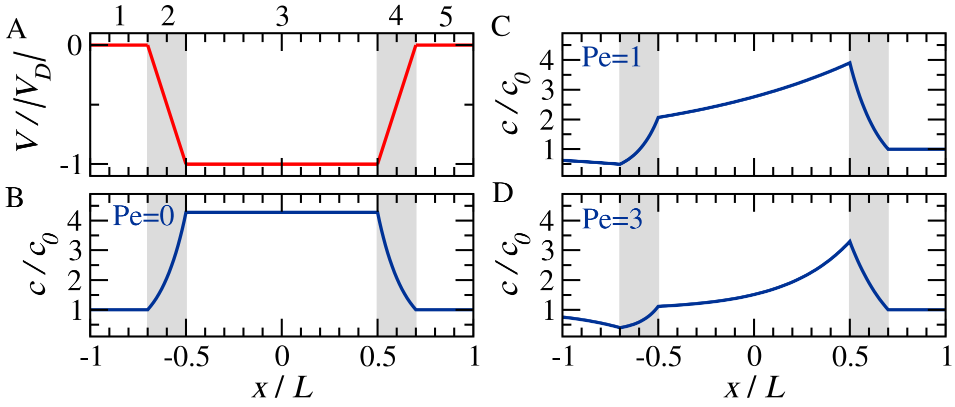


FIG. S3. Potential and concentration profile in the five system regions, respectively the right and left reservoir (1 and 5), the nanochannel (3) and the two transition zones (2 and 4). Both transition zones are highlighted by gray areas. Only a small part of the reservoirs are shown and the size of the transition zones have been increased for visibility. (A): Normalized electric potential $V/|V_D|$, with $V_D$ the potential inside the channel. (B): Concentration profile according to Eq. (6) for $\mathrm{Pe} = 0$ (C): Same as (B) for $\mathrm{Pe} = 1$. (D): Same as (B) for $\mathrm{Pe} = 3$.

length $L_R \gg L$, taken to be one dimensional as well. The probe concentration at the far end of both reservoirs is imposed to be $c_0$. An electrical potential $\phi_\mathrm{D} = V_D \times e/k_BT < 0$, the so-called Donnan potential, is imposed inside the nanochannel. This electrical potential builds up from 0 to $\phi_\mathrm{D}$ within transition regions of extent $\epsilon \ll L, L_R$, which connect the reservoirs and the nanochannel (see Fig. S3 A). In the 1D limit explored here, $\phi_\mathrm{D}$ corresponds to the height-invariant value of the electrical potential. Later on, the impact of a varying potential along $z$ on the experiment's resolution will be discussed.

The solvent moves with a constant velocity $u$ along the axis of the channel. Based on the experimental results presented in the main text, we will consider hereafter effects of finite Peclet number on the dye distribution *i.e.* $\mathrm{Pe} = uL/D \sim 1$. Due to the difference in diffusivities –about one order of magnitude [11, 12]– we will however assume that the salt obeys a zero-Peclet limit. Note that the validity of this assumption is verified below using Finite-Element calculations. Thanks to this hypothesis, the theoretical problem deeply simplifies, allowing to neglect at this level the salt concentration polarization effects and to decouple the electrical potential from the flow.

Under this framework, the dye concentration profile $c$ is obtained in closed form through the stationary convection-diffusion equation that reads

$$\boldsymbol{\nabla} \cdot (-D\boldsymbol{\nabla} c - cD\boldsymbol{\nabla}\phi + \boldsymbol{u}c) = 0, \tag{5}$$

where $D$ is the diffusion coefficient of the probe, $\phi = eV/(k_BT)$ the reduced electrical potential, and where we made use of the fact that the dye is a monovalent cationic species. In the present 1D limit, $\nabla \equiv \partial_x$ and Eq. (5) immediately reduces to

$$\left(\frac{u}{D} - \frac{\partial\phi}{\partial x}\right) c - \frac{\partial c}{\partial x} = \frac{J_0}{D}, \tag{6}$$

where $J_0$ is the total flux of dyes through the channel, which has to be conserved along $x$.See concentration profiles obtained from Eq. (6) in Fig. S3 B C and D for respectively $\mathrm{Pe} = 0$, 1 and 3.

Inside each of the five regions of the system –the (nano)channel, the two reservoirs and transition zones–, the solution for the dye concentration writes

$$c = A_i + B_i \cdot \exp\left(\left(\frac{u}{D} - \frac{\partial\phi}{\partial x}\right) x\right), \tag{7}$$

where $A_i$ and $B_i$ are integration constants, with the index $i$ referring to the areas, respectively $i = 1$ and 5 for the left and right reservoirs, $i = 2$ and 4 for the left and right transition zones and $i = 3$ for the channel. $\partial_x\phi$, the partial derivative of the potential vanishes everywhere but in the transition zones, where it amounts to $\partial_x\phi = \pm\phi_\mathrm{D}/\epsilon$ in the left transition zone ($i = 2$) (resp. right transition zone ($i = 4$)), see Fig. S3 A.

Injecting the five concentration profiles (Eq. (7)) into their respective continuity equations (Eq. (6)), one gets

$$A_1 = A_3 = A_5 = \frac{J_0}{u}, \tag{8}$$

and

$$A_2, A_4 = \frac{\epsilon J_0}{u\epsilon \pm D\phi_D}. \tag{9}$$

Moreover, from the two boundary conditions $c(\pm x_0) = c_0$, where $x_0$ refers to the half length of the total system $x_0 = L/2 + \epsilon + L_R$, one gets using Eq. (7)

$$B_1, B_5 = \left(c_0 - \frac{J_0}{u}\right) e^{\pm u x_0/D}. \tag{10}$$

Finally, from the continuity of the dye concentration at the reservoir-transition zones and the transition zones-nanochannel boundaries, we obtain

$$B_3\, \mathrm{e}^{-uL/(2D)} = (A_2 - A_3) + (A_1 - A_2)\mathrm{e}^{u\epsilon/D}\mathrm{e}^{-\phi_D} + B_1\mathrm{e}^{-\phi_D}\mathrm{e}^{-uL/(2D)}, \tag{11}$$

$$B_3\, \mathrm{e}^{uL/(2D)} = (A_4 - A_3) + (A_5 - A_4)\mathrm{e}^{-u\epsilon/D}\mathrm{e}^{-\phi_D} + B_5\mathrm{e}^{-\phi_D}\mathrm{e}^{uL/(2D)}. \tag{12}$$

In the limit of vanishing transition zones, $\epsilon \to 0$, and accounting for Eqs. (8)–(10), Eqs. (11) and (12) simplify to:

$$B_3\, \mathrm{e}^{-uL/(2D)} = \frac{J_0}{u}\left(\mathrm{e}^{-\phi_D} - 1\right) + \left(c_0 - \frac{J_0}{u}\right)\mathrm{e}^{-\phi_D}\mathrm{e}^{uL_R/D}, \tag{13}$$

$$B_3\, \mathrm{e}^{uL/(2D)} = \frac{J_0}{u}\left(\mathrm{e}^{-\phi_D} - 1\right) + \left(c_0 - \frac{J_0}{u}\right)\mathrm{e}^{-\phi_D}\mathrm{e}^{-uL_R/D}. \tag{14}$$

From the above expressions, $B_3$ can be eliminated to yield the probe flux

$$\frac{J_0}{uc_0} = \frac{\sinh\left(uL/(2D) + uL_R/D\right)}{\sinh\left(uL/(2D) + uL_R/D\right) + \left(\mathrm{e}^{\phi_D} - 1\right)\sinh\left(uL/(2D)\right)}, \tag{15}$$

which further simplifies in the limit of large reservoirs, $L_R \gg L$:

$$\frac{J_0}{uc_0} \simeq 1 + \left(1 - \mathrm{e}^{\phi_D}\right)\frac{\sinh\left(uL/(2D)\right)}{\sinh\left(uL_R/D\right)}. \tag{16}$$

Injecting this expression into Eq. (14) yields the leading order for $B_3$,

$$B_3 \simeq c_0\left(\mathrm{e}^{-\phi_D} - 1\right) e^{-uL/(2D)}. \tag{17}$$

Gathering the previous results for $A_i$ and $B_i$, we eventually obtain the excess dye concentration profile in the reservoirs and in the nanochannel

$$c_1 \simeq c_0 + 2c_0\left(\mathrm{e}^{+\phi_D} - 1\right)\sinh\left(uL/(2D)\right)\mathrm{e}^{ux/D}, \tag{18}$$

$$c_3 \simeq c_0 + c_0\left(\mathrm{e}^{-\phi_D} - 1\right)\mathrm{e}^{-uL/(2D)}\mathrm{e}^{ux/D}, \tag{19}$$

$$c_5 \simeq c_0. \tag{20}$$

Note that in the absence of convection, $u = 0$, one recovers that excess concentration vanishes in both reservoirs while amounting to $c = c_0\mathrm{e}^{-\phi_D}$ in the nanochannel in accordance with the uniformity of the (electro-)chemical potential.

Experimentally, the recorded signal writes

$$\langle c\rangle_{x_1} = \frac{1}{\omega_r}\int_{x_1-\omega_r/2}^{x_1+\omega_r/2} c_3\,\mathrm{d}x, \tag{21}$$

where $\omega_r$ is the radial extent of the confocal volume. With $\omega_r \ll L$, the measurement is essentially punctual so that according to Eq. (19) one gets

$$\langle c\rangle_{x_1} = c_0 + c_0\left(\mathrm{e}^{-\phi_\mathrm{D}} - 1\right)\mathrm{e}^{-uL/2D}\mathrm{e}^{ux_1/D}. \tag{22}$$

Introducing a parameter $\alpha_{1D} = 1/2 - x_1/L$, that account for the position of the spot inside the channel, one can write

$$\langle c\rangle_{x_1} = c_0 + c_0\left(\mathrm{e}^{-\phi_{\mathrm{D}}} - 1\right)\mathrm{e}^{-\alpha_{1D}\mathrm{Pe}}, \tag{23}$$

where $\mathrm{Pe} = uL/D$. Equation (23) reveals the exponential decrease of the local concentration with the flow velocity $u$, and highlights a characteristic velocity

$$u_0 = \frac{D}{\alpha_{1D}L}, \tag{24}$$

that depends on the position of the observation spot $x_1$. Note that the maximum resolution in velocity is $\mathcal{O}(D/L)$ and is obtained at the channel entrance. The resolution in velocity in the center of the channel is $\mathcal{O}(D/(2L))$.

## III. TWO-DIMENSIONAL ANALYTICAL CALCULATION

Here we extend our previous approach to the case where quantities also vary in the $z$ direction, i.e. transverse to the flow. Following equation (6), the stationary convection-diffusion writes

$$\left(\frac{u(x,z)}{D} - \frac{\partial\phi(x,z)}{\partial x}\right)c(x,z) - \frac{\partial c(x,z)}{\partial x} = \frac{J(x,z)}{D}, \tag{25}$$

where the velocity field $u(x,z)$, potential $\phi(x,z)$, concentration $c(x,z)$, and flux $J(x,z)$ are functions of the transverse direction $z$, as well as functions of $x$. In both transition zones, assuming that the potential builds-up linearly, one can write $\partial_x\phi(x,z) = \pm\phi_c(z)/\epsilon$ with $\phi_c(z)$ the potential in the central area. In the following, we do not write explicitly the dependencies in $x$ and $z$.

At equilibrium, $u = 0$ and $J = 0$, we can write from equation (25) that in the left and right transition zones respectively, $\partial_x \ln c = \mp\phi_c/\epsilon$. From there, the equilibrium concentration in the five regions follows:

$$c_1^{(0)} = c_0, \tag{26}$$

$$c_2^{(0)} = c_0\,\mathrm{e}^{-\phi_c\Delta x/\epsilon}, \tag{27}$$

$$c_3^{(0)} = c_0\,\mathrm{e}^{-\phi}, \tag{28}$$

$$c_4^{(0)} = c_0\,\mathrm{e}^{(\Delta x/\epsilon-1)\phi_c}, \tag{29}$$

$$c_5^{(0)} = c_0, \tag{30}$$

where the superscript "(0)" refers to equilibrium solution and where as previously the subscript refers to each of the 5 regions in the system. In the above equations, $\Delta x = x + L/2 + \epsilon$ in the left transition zone #2 and $\Delta x = x - L/2$ in the right transition zone #4.

We now consider the dye concentration in the presence of a small water flux, for which we write down the first correcting term of a Peclet number expansion with Pe defined from the z-averaged velocity $\mathrm{Pe} = \langle u\rangle L/D$. Concentrations in each region thus writes

$$c_i = c_i^{(0)} + \mathrm{Pe}\,c_i^{(1)}(x), \tag{31}$$

while the dye flux is of the form

$$J = \mathrm{Pe}\,J^{(1)}. \tag{32}$$

Injecting Eqs. (31) and (32) into the transport equation (25), one gets for reservoirs

$$c_1^{(1)}(x) = \left(\frac{c_0}{L} - \frac{J_1^{(1)}}{D}\right)(x + L_R + L/2), \quad \text{and} \quad c_5^{(1)}(x) = \left(\frac{c_0}{L} - \frac{J_5^{(1)}}{D}\right)\times(x - L_R - L/2), \tag{33}$$

where we used that $u/\langle u\rangle = 1$ into the reservoirs, that $\epsilon \ll L_R, L$, and that $c_1^{(1)}(x = -L_R - L/2) = c_5^{(1)}(x = L_R + L/2) = 0$. Concerning the central nanochannel, the first order concentration correction is

$$c_3^{(1)}(x) = \left(\frac{c_0}{L}\frac{u\mathrm{e}^{-\phi_c}}{\langle u\rangle} - \frac{J_3^{(1)}}{D}\right)x + B_3, \tag{34}$$

with $B_3$ an integration constant to be calculated.

Now in the transition zones, the solutions simply reads

$$c_2^{(1)} = B_2 \mathrm{e}^{-\phi_c \Delta x/\epsilon} - \frac{J_2^{(1)}}{D}\frac{\epsilon}{\phi_c} + \Delta x \frac{c_0}{L}\frac{u}{\langle u\rangle}\mathrm{e}^{-\phi_c \Delta x/\epsilon}, \tag{35}$$

$$c_4^{(1)} = B_4 \mathrm{e}^{+\phi_c \Delta x/\epsilon} + \frac{J_4^{(1)}}{D}\frac{\epsilon}{\phi_c} + \Delta x \frac{c_0}{L}\frac{u}{\langle u\rangle}\mathrm{e}^{-\phi_c}\mathrm{e}^{\phi_c \Delta x/\epsilon}, \tag{36}$$

where $B_2$ and $B_4$ are integration constants and $\Delta x = x + L/2 + \epsilon$ on the left transition zone and $\Delta x = x - L/2$ on the right transition zone. From the concentration continuity between the regions #1 and #2, one gets

$$B_2 = \left(\frac{c_0}{L} - \frac{J_1^{(1)}}{D}\right) L_R, \tag{37}$$

using $\Delta x = 0$ and $\epsilon \ll L_R, L$. Equivalently, from the concentration continuity between the regions #4 and #5 one gets

$$B_4 = -\left(\frac{c_0}{L} - \frac{J_5^{(1)}}{D}\right) L_R \mathrm{e}^{-\phi_c}. \tag{38}$$

Finally from the continuity between regions #2 and #3 and between #3 and #4, one obtains that $B_3 = 0$, where we have used that solute flux is homogeneous in the reservoirs $J_1^{(1)} = J_5^{(1)} = \langle J^{(1)}\rangle$.

Using again the flux conservation $\langle J_3^{(1)}\rangle = \langle J^{(1)}\rangle$, one gets that $\langle J^{(1)}\rangle \simeq c_0 D/L$ up to terms in $L/L_R \ll 1$. Thus, the averaged concentration in the channel eq. 34 eventually reads

$$\langle c_3\rangle = c_0\langle \mathrm{e}^{-\phi_c}\rangle + \mathrm{Pe}\left[c_0\left(\frac{\langle u\mathrm{e}^{-\phi_c}\rangle}{\langle u\rangle} - 1\right)\frac{x}{L}\right] + \mathcal{O}(\mathrm{Pe}^2). \tag{39}$$

In the 1D case, going back to equations 15, 13 and 14, and taking the limit of Pe $\to 0$ together with $(L_R/L)\mathrm{Pe} \ll 1$, one obtains that the equivalent first order expansion for the dye concentration within the nanochannel writes

$$c_3^{1D} = c_0 \mathrm{e}^{-\phi_D} + \mathrm{Pe}\left[c_0\left(\mathrm{e}^{-\phi_D} - 1\right)\frac{x}{L}\right] + \mathcal{O}(\mathrm{Pe}^2). \tag{40}$$

If we define the Donnan potential $\phi_D$ according to $\mathrm{e}^{-\phi_D} = \langle \mathrm{e}^{-\phi_c(z)}\rangle$, it follows from Eqs. 39 and 40 that the effect of non-uniform velocity and electrostatic potential profiles $u(z)$ and $\phi_c(z)$ within the nanochannel depth can be mapped onto a 1D problem, providing the Peclet number of the 2D problem is renormalized

$$\mathrm{Pe}_{\mathrm{eff.}} = \alpha_{2D}\mathrm{Pe} \quad \text{with} \quad \alpha_{2D} = \frac{\langle u\left(\mathrm{e}^{-\phi_c} - 1\right)\rangle}{\langle u\rangle\langle \mathrm{e}^{-\phi_c} - 1\rangle}, \tag{41}$$

where as stated before, the Peclet number is defined from the averaged velocity $\mathrm{Pe} = \langle u\rangle L/D$.

Now from this mapping in the limit of vanishing flow, we can propose an Ansatz for the nanochannel dye concentration at finite Peclet numbers, including the 2D aspects of the problem. Based on the general solution of the 1D problem for all Peclet, Eq. (19), the approximate 2D dye profiles reads

$$\langle c\rangle_{x_1}^{2D} \simeq c_0 + c_0\left(\langle \mathrm{e}^{-\phi_c}\rangle - 1\right)\mathrm{e}^{-\alpha_{1D}\alpha_{2D}\mathrm{Pe}}, \tag{42}$$

where we recall that $\alpha_{1D} = 1/2 - x_1/L$.

### A. Calculation of $\alpha_{2D}$

Assuming a weak surface potential $\phi_c \ll 1$, $\alpha_{2D}$ writes

$$\alpha_{2D} \approx \frac{\langle u(z)\phi_c(z)\rangle}{\langle u(z)\rangle\langle \phi_c(z)\rangle}. \tag{43}$$

Neglecting the variation of $\phi$ over $x$ (limit $u \to 0$), and using the linearized Poisson-Boltzmann equation, we write the potential profile in a slit nanochannel of height $h$ as

$$\phi_c(z) \approx 2\phi_S \cosh\left(z/\lambda_D\right)\mathrm{e}^{-h/2\lambda_D}, \tag{44}$$

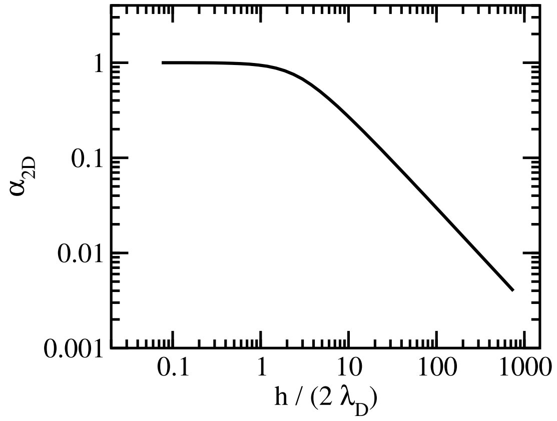


FIG. S4. $\alpha_{2D}$ as a function of $h/(2\lambda_D) = \tilde{h}$ as plotted from Eq. (51).

where we summed the contributions of the two surfaces and where $\phi_S$ stands for the surface potential in $k_BT/e$ unit. The $z$ averaged potential thus reads

$$\langle \phi_c(z) \rangle = \frac{1}{h} \int_{h/2}^{h/2} \phi_c(z) \mathrm{d}z = 2\phi_S \frac{1}{\tilde{h}} \sinh(\tilde{h})\, \mathrm{e}^{-\tilde{h}}, \tag{45}$$

with $\tilde{h} = h/(2\lambda_D)$ the channel height non-dimensionalized with the Debye electrostatic screening length. Note that $\tilde{h} < 1$ corresponds to the regime of double layer overlap and that the limit $\tilde{h} \ll 1$ is the Donnan limit for which one recovers the 1D approach.

Assuming the no-slip boundary condition at the channel walls, the solution for the velocity profile writes

$$u(z) = \frac{1}{\eta} \left( \frac{z^2}{2} - \frac{h^2}{8} \right) \frac{\Delta p}{L}, \tag{46}$$

where the difference of potential $\Delta p$ is defined negative. The velocity averaged over the height $h$ follows as

$$\langle u(z) \rangle = -\frac{h^2}{12} \frac{\Delta p}{\eta L}. \tag{47}$$

Now the z-average of the product $u(z)\phi_c(z)$ writes

$$\langle u(z)\phi_c(z) \rangle = 2\phi_S \left\langle \left( \frac{z^2}{2} - \frac{h^2}{8} \right) \cosh\left(z/\lambda_D\right) \right\rangle \mathrm{e}^{-\tilde{h}} \frac{\Delta p}{\eta L}, \tag{48}$$

and using that

$$\frac{1}{h} \int_{-h/2}^{h/2} \left( \frac{z^2}{2} - \frac{h^2}{8} \right) \cosh(z/\lambda_D) \mathrm{d}z = \lambda_D^2 \left( \sinh(\tilde{h})/\tilde{h} - \cosh(\tilde{h}) \right), \tag{49}$$

we get

$$\langle u(z)\phi_c(z) \rangle = 2\phi_S \lambda_D^2 \left( \sinh(\tilde{h})/\tilde{h} - \cosh(\tilde{h}) \right) \mathrm{e}^{-\tilde{h}} \Delta p/\eta/L. \tag{50}$$

The ratio defining $\alpha_{2D}$ follows as

$$\alpha_{2D} = \frac{\langle u(z)\phi(z) \rangle}{\langle u(z) \rangle \langle \phi(z) \rangle} = \frac{3}{\tilde{h}^2} \left( \tilde{h} \coth(\tilde{h}) - 1 \right), \tag{51}$$

which is a function of $\tilde{h} = h/(2\lambda_D)$ only, see Fig. S4.

## IV. FINITE ELEMENT CALCULATIONS

We used the software Comsol multiphysics to perform finite element calculations. A complete set of equations (Stokes, diffusion-convection and Maxwell) in a 2D geometry is solved with the proper boundary conditions. Details are presented hereafter.

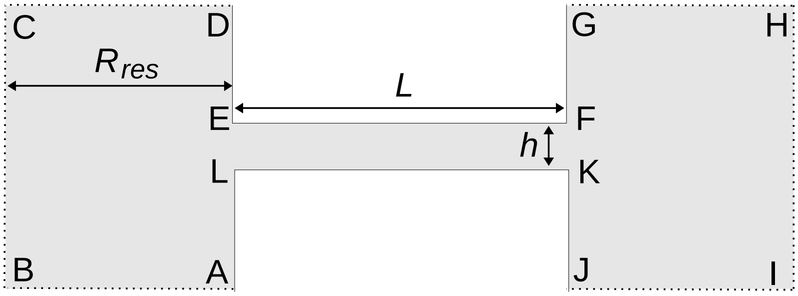


FIG. S5. System used for finite element calculations, see text for the description.

### A. System

We used a system identical to the representation in Fig. S5. A membrane pierced with a nanochannel separates two reservoirs with salt concentration $c_s$ and rhodamine 6G concentration $c_r$. The nanochannel is a slit with height $h = 150\,\mathrm{nm}$ and a length $L = 3\,\mu\mathrm{m}$. Note that the length of the system must be long enough to ensure a small lateral Peclet number, $uh/D \ll 1$. The channel is charged with a surface charge $\Sigma = -1\,\mathrm{mC/m^2}$. The characteristic size $R_{\mathrm{res}} = 100\,\mu\mathrm{m}$ of the reservoirs is taken to be larger than the Duhkin length $\ell_{\mathrm{Du}}$, the Debye length $\lambda_D$ and $h$ in order to avoid finite size effects [13, 14].

### B. Hydrodynamics

We solve the Stokes equation for an incompressible flow $\boldsymbol{\nabla} \cdot \mathbf{u} = \mathbf{0}$

$$\eta \Delta \boldsymbol{u} = \boldsymbol{\nabla} p - \mathbf{F}_{\mathrm{elec}}, \tag{52}$$

where $\mathbf{u}$ is the water velocity field, $p$ the pressure field, $\mathbf{F}_{\mathrm{elec}}$ an electric volume force equal to

$$\mathbf{F}_{\mathrm{elec}} = -\mathcal{F}(c_+ - c_-)\boldsymbol{\nabla} V, \tag{53}$$

with $\mathcal{F}$ the Faraday constant, $c_\pm$ the concentration in $\pm$ species and $V$ the electrical potential. A pressure equal to $\Delta p + p_{\mathrm{atm}}$ is imposed along A-B-C-D and $p_{\mathrm{atm}}$ is imposed along G-H-I-J (see Fig. S5). The no-slip boundary condition is imposed along walls D-E-F-G and J-K-L-A.

### C. Electrostatics

We solve the Maxwell-Gauss equation

$$\boldsymbol{\nabla} \cdot \mathbf{D} = \rho, \tag{54}$$

together with a constitutive relation relating the electric displacement $\mathbf{D}$ with the electric field $\mathbf{E}$:

$$\mathbf{D} = \epsilon_0 \epsilon_r \mathbf{E}. \tag{55}$$

$\epsilon_r$ is the dimensionless relative permittivity, and $\epsilon_0$ the vacuum permittivity and $\rho$ the space charge density: $\rho = \mathcal{F}(c_+ - c_-)$. The relationship between electric potential $V$ and the electric field $\mathbf{E}$ is

$$\mathbf{E} = -\boldsymbol{\nabla} V. \tag{56}$$

A surface charge $\Sigma$ is applied along E-F and K-L, see Fig. S5. The no-charge boundary condition is set on D-E, F-G, J-K and L-A. The electrical potential $V = 0$ is imposed along A-B-C-D, and a floating potential condition is applied along G-H-I-J.

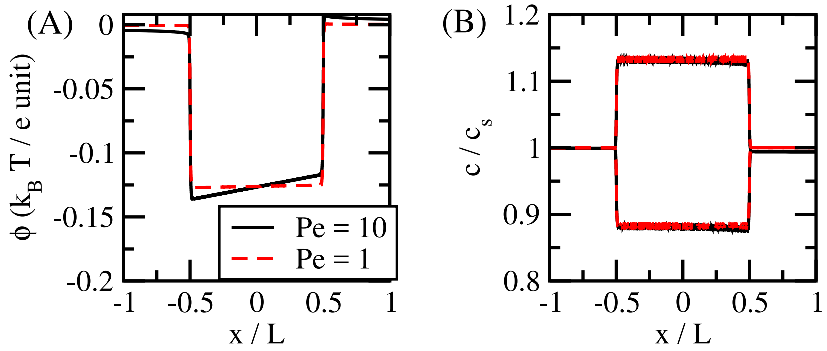


FIG. S6. Profiles along the central line of the channel, i.e. $z = 0$, for Pe = 1 and Pe = 10, as extracted from Finite Element calculations. Potential profile **(A)** and salt concentration profiles **(B)**.

### D. Transport of diluted species for salt

Solute species concentration are solved through the Nernst-Planck equation. The molar flux for both salt species of respective concentration $c_\pm$ is defined as

$$\boldsymbol{J}_\pm = -D_s \left[ \boldsymbol{\nabla} c_\pm \pm \frac{eD_s}{k_B T} c_\pm \boldsymbol{\nabla} V \right] + \boldsymbol{u} c_\pm, \tag{57}$$

where $D_s = 1 \cdot 10^{-9}\,\mathrm{m}^2/\mathrm{s}$. Note that the convective term $\boldsymbol{u}c_\pm$ is turned off if not specified otherwise. The molar flux is conserved, i.e., it obeys the Nernst-Plank condition

$$\boldsymbol{\nabla} \cdot \boldsymbol{J}_\pm = 0. \tag{58}$$

The no-flux boundary condition ($-\boldsymbol{n} \cdot \boldsymbol{J}_\pm = 0$) was imposed along D-E-F-G and J-K-L-A, and the concentration $c_s$ was imposed for both species along A-B-C-D and G-H-I-J, see Fig. S5.

### E. Transport of diluted species for dye

The dye concentration is handled along the same line as previously described for the salt. The molar flux for the dye of concentration $c$ is defined as

$$\boldsymbol{J} = -D \left[ \boldsymbol{\nabla} c + \frac{eD}{k_B T} c \boldsymbol{\nabla} V \right] + \boldsymbol{u} c, \tag{59}$$

and obeys the Nernst-Plank condition

$$\boldsymbol{\nabla} \cdot \boldsymbol{J} = 0, \tag{60}$$

where $D = 4 \cdot 10^{-10}\,\mathrm{m}^2/\mathrm{s}$. The no-flux boundary condition ($-\boldsymbol{n} \cdot \boldsymbol{J} = 0$) was imposed along D-E-F-G and J-K-L-A, and the concentration $c_s$ was imposed for both species along A-B-C-D and G-H-I-J, see Fig. S5.

### F. Validity of the zero-Peclet assumption for salt

Using the previously described finite-element calculation, we solve the concentration, velocity and potential profiles for a surface charge $\Sigma = -1\,\mathrm{mC/m}^2$, $c_s = 10^{-6}\,\mathrm{M}$, $h = 150\,\mathrm{nm}$ and $2\lambda/h = 4$. The convective term $\boldsymbol{u}c_\pm$ in Eq. (57) is turned on. Both electrical potential and salt concentration profiles along the axis of the channel are given for a peclet number $\mathrm{Pe} = uL/D = 1$ and 10, where $u$ is the average fluid velocity, see figure S6. For Pe = 10, the value of the potential deviates from its equibrium value by less than 6%, and the salt concentration by less than 1%. These results validate the assumption of a salt concentration that remains unperturbed by the flow within the chosen range of Peclet numbers.

## V. EFFECT OF REVERSIBLE ADSORPTION ON DETECTION RESOLUTION

Here we use a home-made Matlab code to solve the diffusion and convection of a single particle inside a nanochannel with absorbing walls in order to explore the impact of the reversible adsorption of dye on the resolution of the present method. When the particle encounter a channel wall, it adsorbs with a probability $p_{\rm ads} = 0.02$. Once adsorbed, the particle is immobile for an exponentially distributed duration of mean 100 ms. This parameters are chosen in order to obtain a correlation function that reproduce roughly the correlation function obtained in the present experiment. The system accessible for diffusion is a channel of length $L$ and height $h$, connected to reservoirs of size $R_{\rm res}$, as depicted in Fig. S5. Apart when adsorbed in surface, the particle follows the diffusion-convection equation, where the velocity field $\mathbf{u}$ has been previously calculated using Finite Element, as described in subsection IV B, see an example in Fig. S7. An attractive potential is added to the particle inside the channel, mimicking an electrical Donnan potential corresponding to a full overlap of Electrical Double Layers $V(z) = V_s \times \mathrm{rect}(x/L)$, with rect() the rectangular function with smoothing ensuring the absence of potential inside the reservoir and a smooth transition at the entrances of the channel. The number of particle averaged over time $n_{\rm tot}$ inside a finite spot located in the central part of the channel and mimicking the confocal detection volume is extracted. As observed in Fig. S7, while the adsorption increases the average number of particle inside the confocal volume, no change in the resolution in velocity is observed.

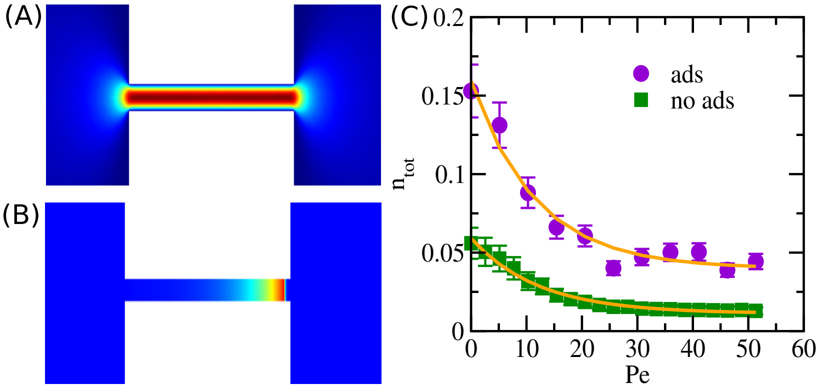


FIG. S7. **(A)** Example of velocity profile in a nanochannel, color-scale is the norm of the velocity from blue, low velocity, to red, high velocity. **(B)** Example of density profile with a Peclet number equal to 5. **(C)** Evolution of the average total number detected in the confocal volume located at the center of the channel as a function of the Peclet number Pe. Symbol are results from numerical simulation and the continuum line is an exponential fit $y = a\exp(-x/b) + c$, with $b = 12.1$ in absence of adsorption and $b = 11.6$ in presence of adsorption. Error bars correspond to standard deviation.

[1] Fabien Chauvet, Sandrine Geoffroy, Abdelkrim Hamoumi, Marc Prat, and Pierre Joseph, "Roles of gas in capillary filling of nanoslits," Soft Matter **8**, 10738–10749 (2012).
[2] Thomas B. Sisan and Seth Lichter, "The end of nanochannels," Microfluidics and Nanofluidics **11**, 787–791 (2011).
[3] R. A. Sampson, "On Stokes's Current Function," Philosophical Transactions of the Royal Society A: Mathematical, Physical and Engineering Sciences **182**, 449–518 (1891).
[4] Simon Gravelle, Laurent Joly, Christophe Ybert, and Lydéric Bocquet, "Large permeabilities of hourglass nanopores : From hydrodynamics to single file transport," The Journal of Chemical Physics **141**, 18C526 (2014).
[5] Elke Haustein and Petra Schwille, "Fluorescence correlation spectroscopy: novel variations of an established technique," Annu. Rev. Biophys. Biomol. Struct. **36**, 151–169 (2007).
[6] O Krichevsky and G Bonnet, "Fluorescence correlation spectroscopy: the technique and its applications," Rep. Prog. Phys. **65**, 251 (2002).
[7] Jason D Fowlkes and C Patrick Collier, "Single-molecule mobility in confined and crowded femtolitre chambers." Lab on a chip **13**, 877–85 (2013).
[8] Charlisa R. Daniels, Carmen Reznik, and Christy F. Landes, "Dye diffusion at surfaces: Charge matters," Langmuir **26**, 4807–4812 (2010).
[9] Harishanker Patel, Mahesh K. Swami, Asmita Malik, Pankaj K. Kushwaha, S. S. Raja, and Pradeep K. Gupta, "Effect of surface interactions on diffusion of molecules: Fluorescence correlation spectroscopic investigation," in International Conference on Fibre Optics and Photonics (Optical Society of America, 2012) p. T1A.3.
[10] N. F Y Durand, Claudio Dellagiacoma, Raphaël Goetschmann, Arnaud Bertsch, Iwan Märki, Theo Lasser, and Philippe Renaud, "Direct observation of transitions between surface-dominated and bulk diffusion regimes in nanochannels," Analytical

Chemistry **81**, 5407–5412 (2009).

[11] H. Harned and R. L. Nuttall, "The Diffusion Coefficient of Potassium Chloride in Dilute Aqueous Solution," J. Am. Chem. Soc. **69**, 736–740 (1947).

[12] Christopher T Culbertson, Stephen C Jacobson, and J Michael Ramsey, "Diffusion coefficient measurements in microfluidic devices." Talanta **56**, 365–73 (2002).

[13] Lydéric Bocquet and Elisabeth Charlaix, "Nanofluidics, from bulk to interfaces," Chemical Society Reviews **39**, 1073–1095 (2010).

[14] Choongyeop Lee, Laurent Joly, Alessandro Siria, Anne Laure Biance, Rémy Fulcrand, and Lydéric Bocquet, "Large apparent electric size of solid-state nanopores due to spatially extended surface conduction," Nano Letters **12**, 4037–4044 (2012).
